# Supplementary material for: The menu complexity of "one-and-a-half-dimensional" mechanism design
Source: arXiv:1711.02165 source file (2017-11-06)
Supplement: Supplementary file 1 [file appendix.tex]

\section{Appendix}
\label{sec:appendix}
